# Supplementary material for: Hinge-like structure induced unusual properties of black phosphorus and new strategies to improve the thermoelectric performance
Source: arXiv:1406.0261 source file (2014-10-29)
Supplement: Supplementary file 1 [file SupplementalInformation.pdf]

## Supplemental Information

# Hinge-like structure induced unusual properties of black phosphorus and new strategies to improve the thermoelectric performance

Guangzhao Qin,[1] Qing-Bo Yan,[1,*] Zhenzhen Qin,[2] Sheng-Ying Yue,[3]
Hui-Juan Cui,[3] Qing-Rong Zheng,[3] and Gang Su[3,†]

[1]*College of Materials Science and Opto-Electronic Technology,*
*University of Chinese Academy of Sciences,*
*Beijing 100049, People's Republic of China*

[2]*College of Electronic Information and Optical Engineering,*
*Nankai University, Tianjin 300071, People's Republic of China*

[3]*School of Physics, University of Chinese Academy of Sciences,*
*Beijing 100049, People's Republic of China*

## I. ANALOGY BETWEEN SnSe AND BLACK PHOSPHORUS

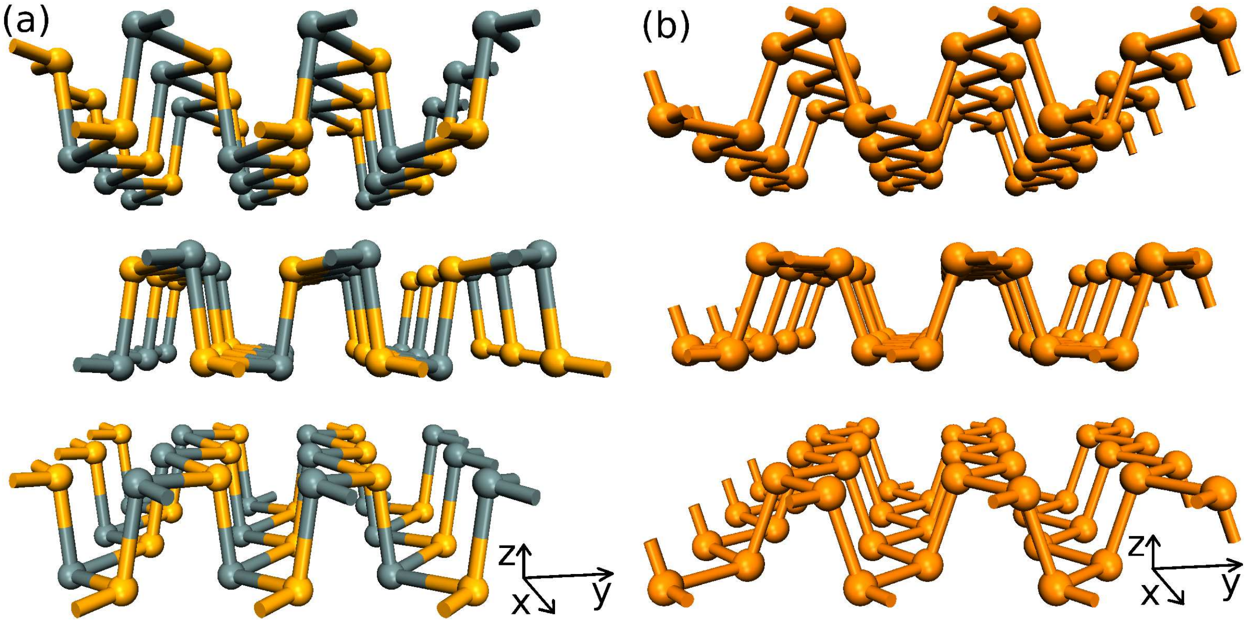


FIGURE S 1. Perspective view of (a) SnSe and (b) black phosphorus.

As shown in Fig. S1, black phosphorus (BP) has an almost same hinge-like layered structure as SnSe. BP has a higher symmetry with the *Cmca* (No. 64) space group, while SnSe crystal has lower symmetry with *Pnma* (No. 62) space group in the reason of two types of atoms.

## II. GEOMETRICAL STRUCTURE OF BLACK PHOSPHORUS

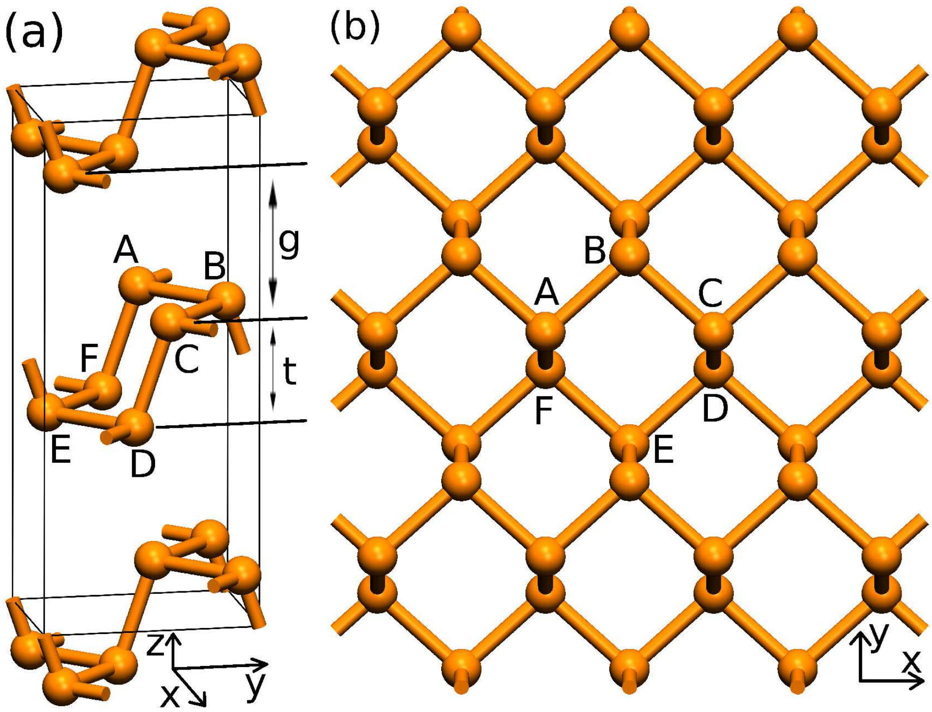


FIGURE S 2. (a) A conventional cell of the crystal structure of black phosphorus and (b) a top view of monolayer. Within a hexagonal ring in one single layer, the upper three atoms are indicated as $A$, $B$ and $C$, while the nether three atoms are indicated as $D$, $E$ and $F$. Layer thickness $t$ is defined as the vertical distance between upper atoms and neither atoms in one single layer, and inter-layer distance $g$ is defined as the separation between two single layers. The lattice constants along $x$, $y$ and $z$ directions are defined as $a$, $b$ and $c$, respectively.

The crystal structure of bulk BP (Fig. S2) is optimized with different functionals, and the lattice constants are summarized in Table SI. For results obtained from PBE functional[1], the lattice constants $a$ and $b$ are slightly underestimated and overestimated, respectively, while $c$ and $\angle$BCD are significantly overestimated. Note that lattice constant $c$ is related to the layer thickness and inter-layer distance, the above overestimation may due to the lack of the consideration of *van der Waals* interactions. Thus the vdW-DF level with optB88 for exchange functional (optB88-vdW)[2,3] is adopted to take *Van der Waals* interactions into account, and more reasonable lattice constants are obtained, as listed in Table SI, which also agrees well with the results from Ji et. al.[4].

The calculated elastic constants within the functional optB88-vdW and the results from

TABLE S I. Lattice constants and structure parameters of bulk black phosphorus from computational and experimental results.

| Functional | $a$(Å) | $b$(Å) | $c$(Å) | AB(Å) | CD(Å) | ∠ABC(°) | ∠BCD(°) |
|---|---|---|---|---|---|---|---|
| optB88-vdW | 3.342 | 4.468 | 10.719 | 2.246 | 2.280 | 96.183 | 102.420 |
| PBE | 3.306 | 4.564 | 11.291 | 2.224 | 2.261 | 95.990 | 103.589 |
| PW91[a] | 3.348 | 4.422 | 10.578 | 2.238 | 2.261 | 96.85 | 102.31 |
| Exp.[b] | 3.3133 | 4.374 | 10.478 | 2.224 | 2.277 | 96.34 | 102.09 |

[a] Reference[5]
[b] Reference[6]

previous computation and experiment are collected as shown in Table SII. The calculated elastic constants satisfy Born's mechanical stability criteria and are in good agreement with experimental values and previous computational results, implying the mechanical stability of the optimized structure of BP.[7–9] The elastic constants $C_{11}$, $C_{22}$ and $C_{33}$ are directly related to the sound propagation along the lattice direction $x$, $y$ and $z$, respectively, reflecting the stiffness to uniaxial strain. It is shown that BP with a large elastic constant $C_{11}$ is much harder along $x$ direction than along $y$ and $z$ directions, which coincides with the Young's modulus as illustrated in the main article.

TABLE S II. Elastic constants of bulk black phosphorus from computational and experimental results.

| Functional | $C_{11}$ | $C_{22}$ | $C_{33}$ | $C_{44}$ | $C_{55}$ | $C_{66}$ | $C_{12}$ | $C_{13}$ | $C_{23}$ |
|---|---|---|---|---|---|---|---|---|---|
| optB88-vdW | 179.3 | 52.5 | 45.5 | 55.6 | 3.9 | 12.7 | 38.9 | 6.3 | 0.07 |
| PBE-Grimme[a] | 191.9 | 52.3 | 73.0 | 25.5 | 8.8 | 63.6 | 40.8 | 8.3 | 0.6 |
| Exp.[b] | 178.6 | 55.1 | 53.6 | 21.3, 11.1 | 5.5 | 14.5, 15.6 | - | - | - |
| Exp.[c] | 284 | 80 | 57 | 17.2 | 10.8 | 59.4 | - | - | - |

[a] Reference[7]
[b] Reference[8]
[c] Reference[9]

To reveal the effect of strain on one single layer inside bulk BP, the interlayer distance

$g$ and layer thickness $t$ are also extracted as shown in Fig. S3 (note the different scales of $t$ and $g$). When strain along $x$ direction varies from $-10\%$ (compressive) to 10% (tensile), the interlayer distance $g$ decreases gradually, while the layer thickness $t$ firstly decreases and then increases, which could be ascribed to the firstly decrease and then increase of the dihedral angle formed by plane $ACD$ and $ABC$. The layer thickness $t$ gets a minimum when the compressive strain along $x$ direction reaches $-3\%$, then increases almost linearly with tensile strain. If strain is applied along $y$ direction, interlayer distance $g$ increases and layer thickness $t$ decreases with strain varies from compressive to tensile as shown in Fig. S3(b). When strain is applied along $z$ direction as shown in Fig. S3(c), the interlayer distance $g$ increases almost linearly as the strain varies from compressive to tensile, while the layer thickness $t$ increases and then decreases, i.e., there is a maximum of layer thickness $t$ and it appears with a tensile strain of 4% applied, which might be ascribed to the interlayer *van der Waals* interactions. When a tiny tensile strain is applied, the interlayer *van der Waals* interactions would contribute an attraction between layers, resulting in the increase of layer thickness $t$. If the tensile strain continues increasing and exceeds 4%, the interlayer *van der Waals* interactions would become weaker, and then the layer thickness $t$ falls back. The layer thickness $t$ would be expected to converges to the thickness of freestanding monolayer BP, which is obtained as 2.13 Å by carefully optimized the geometric structure of monolayer BP.

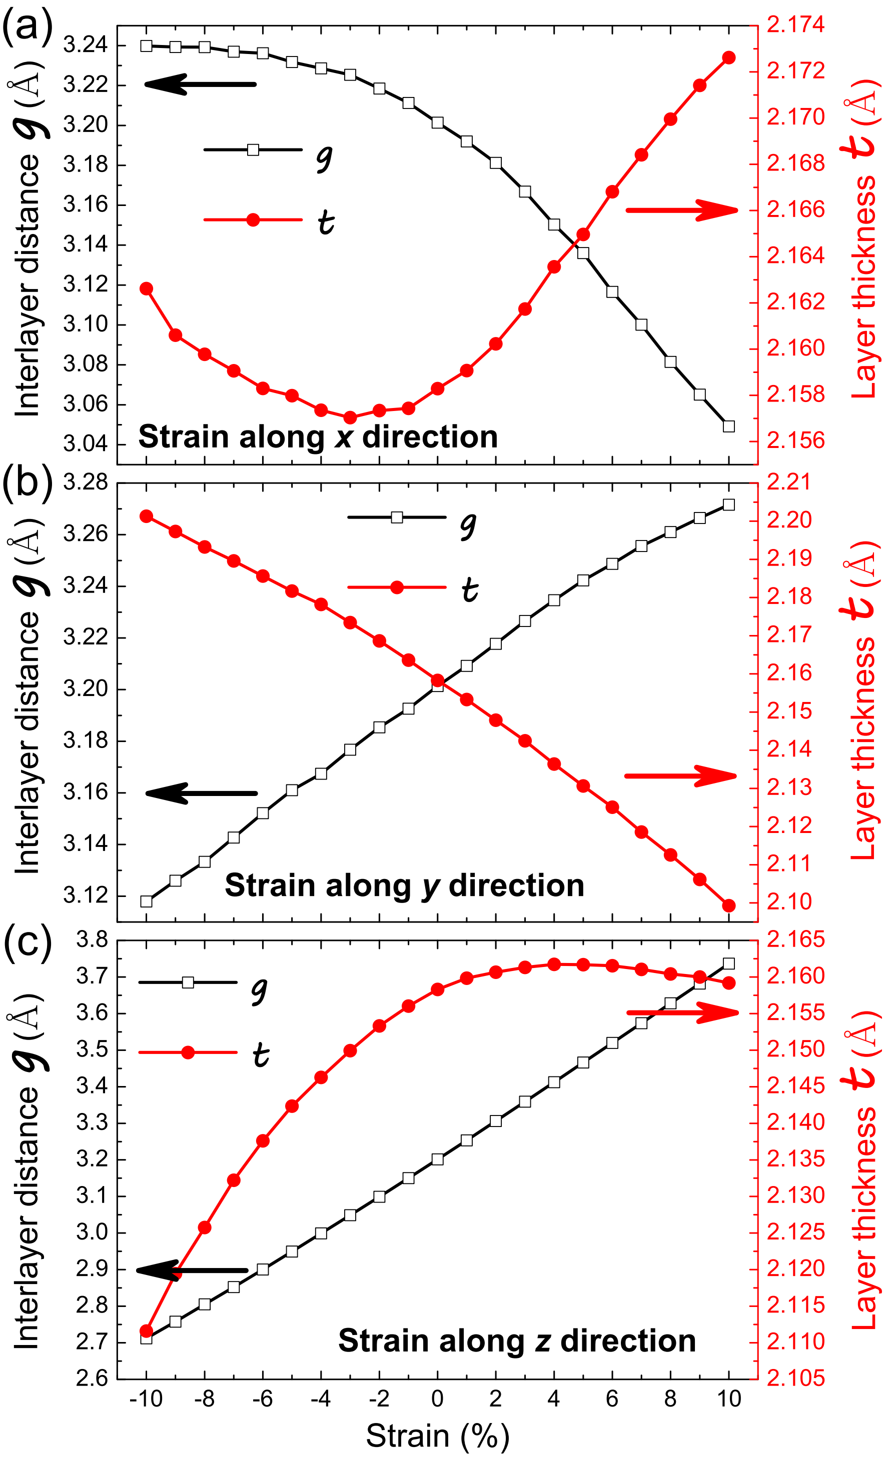


FIGURE S 3. Inter-layer distance $g$ (left in black) and layer thickness $t$ (right in red) versus strain along (a) $x$, (b) $y$ and (c) $z$ direction. Strain is defined as $s = (l - l_0)/l_0$, where $l = a, b, c$, are lattice parameters along $x, y, z$ directions under strain, and $l_0 = a_0, b_0, c_0$, are the lattice constants without strain.

## III. ELECTRONIC STRUCTURE OF BLACK PHOSPHORUS UNDER STRAIN

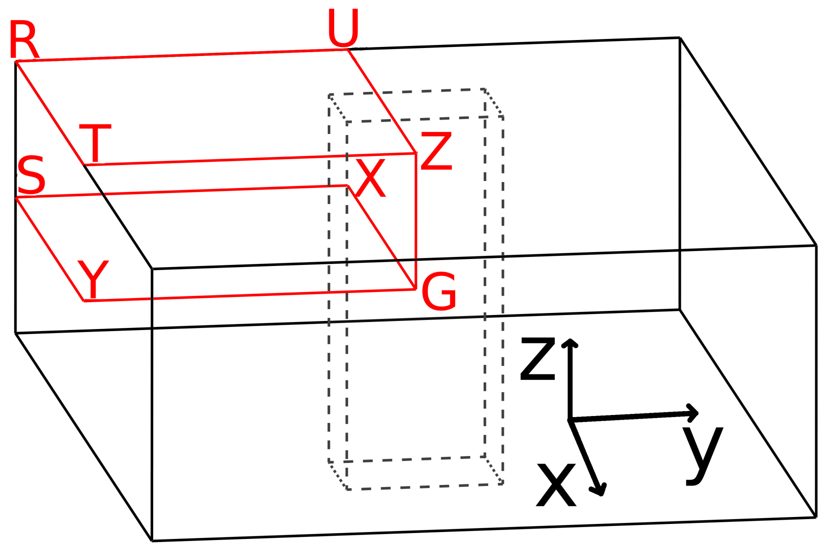


FIGURE S 4. The high-symmetry $k$-points in Brillouin zone. The dashed line indicates the conventional unit cell of bulk black phosphorus.

In order to obtain the anisotropic properties of BP along three different lattice directions, we use the conventional unit cell but not primitive cell for the calculations of band structures and the thermoelectric properties. The high symmetry $k$-points in corresponding Brillouin zone are indicated as G(Γ), X, S and Y, etc., and the path of $k$-points used for band structure calculation are shown in Fig. S4.

As the exact band gap is important for the accurate prediction of the thermoelectric (TE) transport properties, the electronic structures are calculated at modified Becke-Johnson (mBJ) level[10]. Fig. S5 indicates the energy band structures and density of states (DOS) without strain and with several strains applied along $x$, $y$, and $z$ directions, from which the transitions among metal, direct and indirect band gap semiconductor can be explained.

As described in main article, when tensile strain is applied along $x$ direction, the band gap $E_g$ firstly keeps direct and increases almost linearly, but then turns into indirect when the tensile strain reaches 8%. It could be explained by the descent of the conduction band between $Y$ and $\Gamma$ point, and the concurrent ascent of the valence band at the adjacent area between $Y$ and $\Gamma$ point, as indicated by arrows in Fig. S5(a). When strain is along $y$ direction, the transition from direct to indirect of band gap occurs at 3% tensile strain, which could be attributed to the slower ascent of the conduction band between $Z$ and $U$

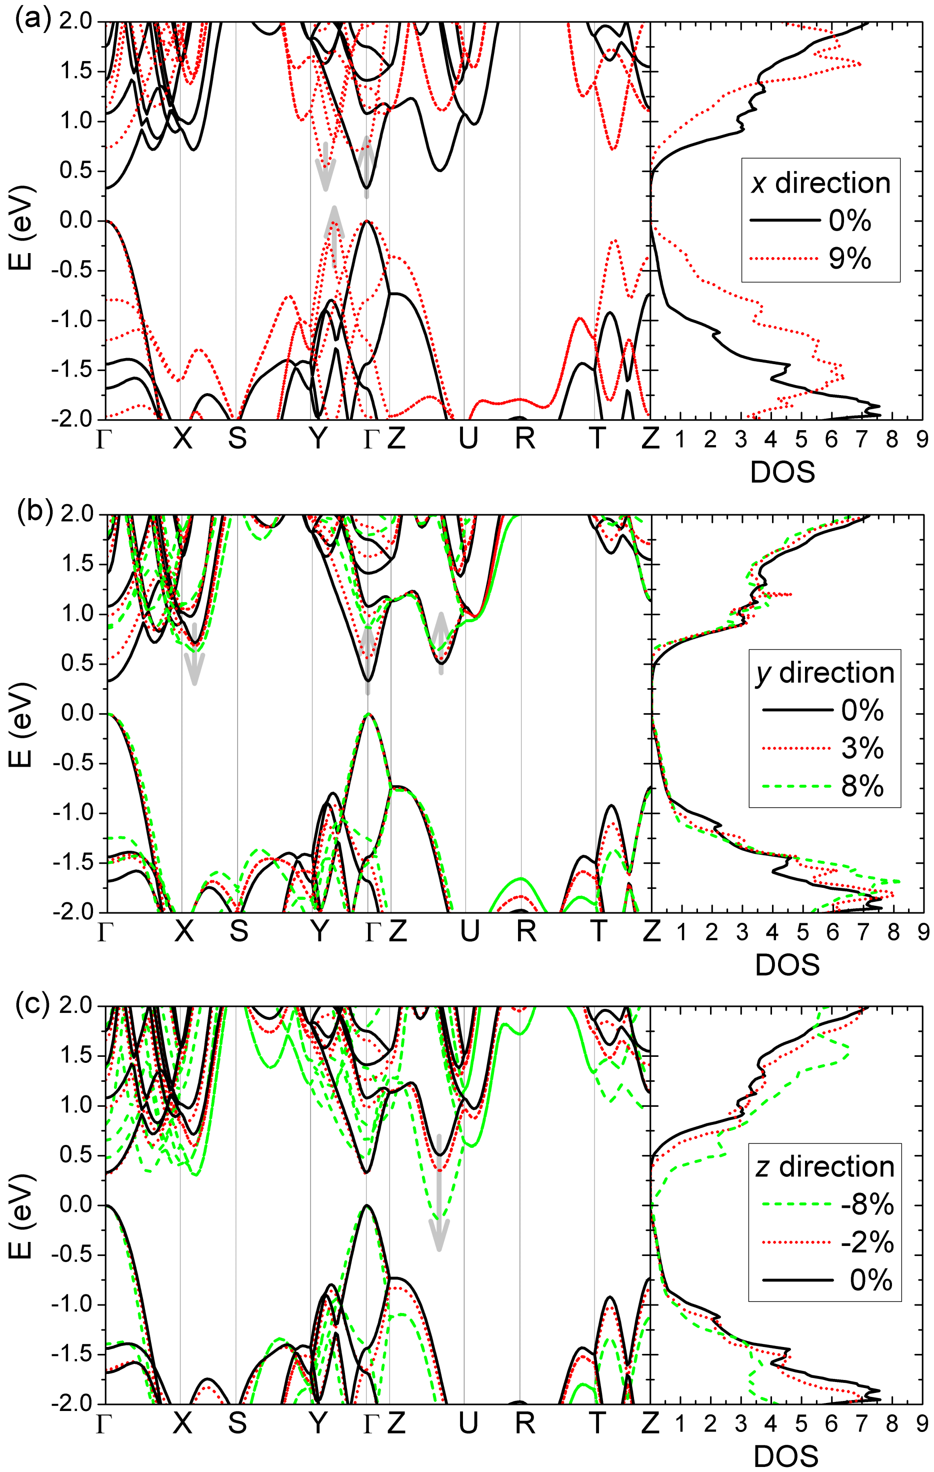


FIGURE S 5. Calculated electronic band structures and density of states (DOS) of black phosphorus (BP) without and with typical strains applied along (a) $x$, (b) $y$ and (c) $z$ directions. The valence band maximums are shifted to zero. The arrows indicate the ascend or descend of bands caused by strain.

than that at $\Gamma$ point, as shown in Fig. S5(b). Note the concurrent descent of the conduction band between $X$ and $S$, which becomes conduction band minimum (CBM) when the tensile strain reaches 8%, leading to the decrease of the indirect band gap. As shown in Fig. S5(c), with the increasing compressive strain along $z$ direction, the conduction band between $Z$ and $U$ descends and then becomes the new CBM when the compressive strain reaches $-3\%$, leading to the transition of BP into an indirect band gap semiconductor, and the indirect gap decreases steeply with the compressive strain. When the compressive strain reaches $-7\%$, the band gap becomes zero and BP transits into metal eventually. The enhancement on $ZT$ of BP under strain could be also rationalized by considering of the strain effect on the band structures and DOS, as discussed in main article.

## IV. SEEBECK COEFFICIENTS $S$ AND $ZT$ VALUES OF BLACK PHOSPHORUS ALONG $y$ AND $z$ DIRECTIONS

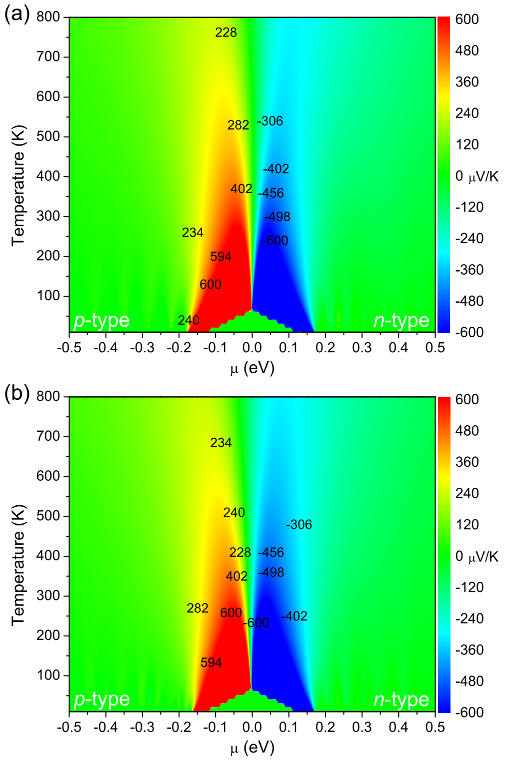


FIGURE S 6. The thermopower ($S$) along (a) $y$ and (b) $z$ directions as functions of chemical potential ($\mu$) and temperature $T$.

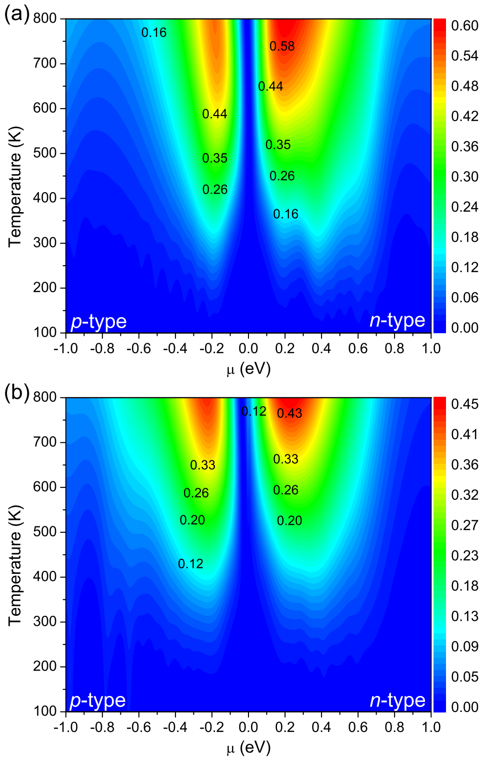


FIGURE S 7. The $ZT$ along (a) $y$ and (b) $z$ directions as functions of chemical potential ($\mu$) and temperature $T$.

The thermopower (S) and $ZT$ along $y$ and $z$ directions shown in Fig. S6 and Fig. S7 as functions of chemical potential ($\mu$) and temperature $T$. The major features are similar to that along $x$ direction (see Fig. 4 and Fig. 5 in main article).

## V. THERMOPOWER ($S$) AT 300 K AND 500 K

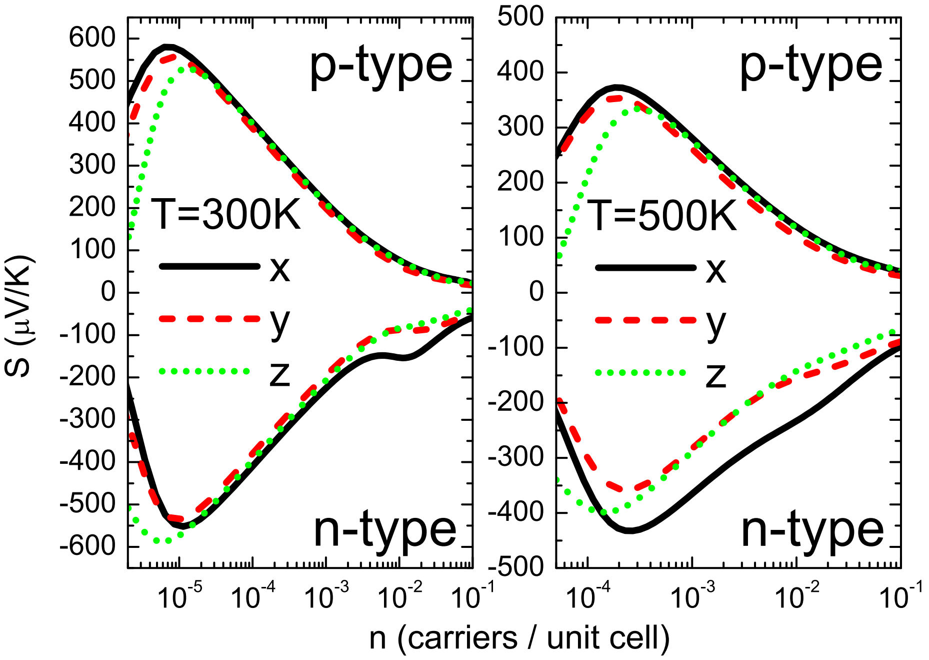


FIGURE S 8. Thermopower ($S$) along $x$, $y$ and $z$ directions as a function of doping level at 300 K and 500 K.

The thermopower ($S$) at 300 K and 500 K are shown in Fig. S8. Along with the increasing temperature, the anisotropic performance of thermopower becomes obviously, especially for electron ($n$-type) doping. The doping level is obtained by integrating the DOS of the system[11].

## VI. TEMPERATURE EFFECTS ON $ZT$ MAXIMUMS

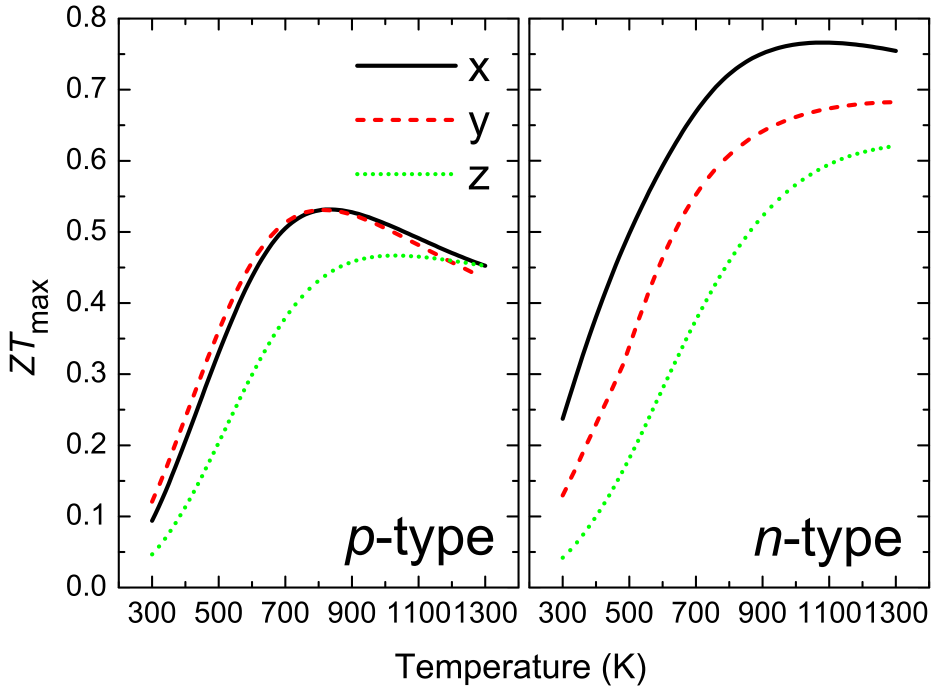


FIGURE S 9. The $ZT$ maximums along $x$, $y$ and $z$ directions as a function of temperature for both hole ($p$-type) and electron ($n$-type) doped black phosphorus.

Fig. S9 shown the $ZT$ maximums along $x$, $y$ and $z$ directions at each temperature are determined by optimizing doping level for both hole ($p$-type) and electron ($n$-type) doped BP, respectively. The temperature for the best TE performance along $y$ direction is 810 K for the hole ($p$-type) doped BP, and higher for electron ($n$-type) doping or along other directions, hence BP is indeed a TE material working at medium-high temperature. At the same time, considering the thermodynamic stable temperature and melting temperature of BP as 823 K and 883 K[6,12], we only concern the TE performance of BP up to 800 K.

## VII. RELAXATION TIME OF CARRIERS IN BLACK PHOSPHORUS

The relaxation time $\tau$ can be derived from the relation $\tau = \mu m^*/e$, where $\mu$ is carrier mobility, $m^*$ is the effective mass of carrier, and $e$ is the elementary charge. With $\mu$ and $m^*$ along different lattice directions for both electron ($n$-type) and hole ($p$-type) doped BP extracted from experiment[6], the anisotropic $\tau$ for BP can be evaluated as shown in Table SIII.

TABLE S III. The carrier mobility ($\mu$), effective mass of carrier ($m^*$), and the calculated scattering time ($\tau$) along three different lattice directions for both electron ($n$-type) and hole ($p$-type) doped black phosphorus.

| doping type | direction | $\mu(\mathrm{cm^2/V\cdot s})^{\mathrm{a}}$ | $m^*/m_0{}^{\mathrm{a}}$ | $\tau(10^{-13}\,\mathrm{s})$ |
|---|---|---|---|---|
| $n$-type | $x$ | 460 | 1.027 | 2.686 |
| | $y$ | 2300 | 0.0826 | 1.080 |
| | $z$ | 400 | 0.128 | 0.291 |
| $p$-type | $x$ | 1200 | 0.648 | 4.421 |
| | $y$ | 3000 | 0.076 | 1.296 |
| | $z$ | 540 | 0.280 | 0.860 |

[a] Reference[6]

* yan@ucas.ac.cn

† gsu@ucas.ac.cn; http://tcmp2.ucas.ac.cn/

1 Perdew, J.P., Burke, K. & Ernzerhof, M. Generalized gradient approximation made simple. *Phys. Rev. Lett.*, **77**, 3865-3868 (1996).

2 Klimes, J., Bowler, D.R., and Michaelides, A. Van der waals density functionals applied to solids. *Phys. Rev. B*, **83**, 195131 (2011).

3 Klimes, J., Bowler, D.R., and Michaelides, A. Chemical accuracy for the van der waals density functional. *J. Phys.: Condens. Matter*, **22**, 022201 (2010).

[4] Qiao, J., Kong, X., Hu, Z.-X., Yang, F. & Ji, W. High-mobility transport anisotropy and linear dichroism in few-layer black phosphorus. *Nat. Commun.* **5**, 4475 (2014).

[5] Du, Y., Ouyang, C., Shi, S. & Lei, M. Ab initio studies on atomic and electronic structures of black phosphorus. *J. Appl. Phys.*, **107**, 093718 (2010).

[6] Morita, A. Semiconducting black phosphorus. *Appl. Phys. A*, **39**, 227-242 (1986).

[7] Appalakondaiah, S., Vaitheeswaran, G., Lebègue, S., Christensen, N. E. & Svane, A. Effect of van der Waals interactions on the structural and elastic properties of black phosphorus. *Phys. Rev. B* **86**, 035105 (2012).

[8] Kzuki, Y., Hanayama, Y., Kimura, M., Nishitake, T. & Endo, S. Measurement of Ultrasound Velocity in the Single Crystal of Black Phosphorus up to 3.3 GPa Gas Pressure. *J. Phys. Soc. Jpn.* **60**, 1612-1618 (1991).

[9] Yoshizawa, M., Shirotani, I. & Fujimura, T. Thermal and Elastic Properties of Black Phosphorus. *J. Phys. Soc. Jpn.* **55**, 1196-1202 (1986).

[10] Tran, F. & Blaha, P. Accurate band gaps of semiconductors and insulators with a semilocal exchange-correlation potential. *Phys. Rev. Lett.*, **102**, 226401 (2009).

[11] Madsen, G.K.H. & Singh, D.J. BoltzTraP. a code for calculating band-structure dependent quantities. *Comput. Phys. Commun.*, **175**, 67-71 (2006).

[12] Warschauer, D. Electrical and optical properties of crystalline black phosphorus. *J. Appl. Phys.*, **34**, 1853-1860 (1963).
